# Supplementary material for: Integral Fast Fourier Color Constancy
Source: arXiv:2502.03494 source file (2025-02-05)
Supplement: Supplementary file 1 [file X_suppl.tex]

\clearpage
\setcounter{page}{1}
\setcounter{section}{0}
\maketitlesupplementary

\section{Data Augmentation}
During training, the most straightforward input is the log-chroma histogram of an image. However, this approach overlooks spatial information and does not utilize additional sources of information, such as edges or spatial neighborhood relationships. In the main paper, we estimate the most accurate illumination \( L \) by filtering a set of histograms \( {N} \) constructed from the log-chroma values and local absolute deviation metrics of the pixels in the image \( I \). 

Beyond this, the model can also process a set of histograms \(\{N_j\}\) derived from a group of "augmented" images \(\{I'_j\}\). The filtered responses of these histograms are aggregated and passed through a softmax function to compute probabilities. These augmented images incorporate edge and spatial statistical information from \( I \), enabling the model to leverage multiple information sources.

It is important to note that the chroma histograms must maintain a precise mapping between channel scaling in the input image and shifts in histogram space. As a result, augmented images must be non-negative and preserve intensity scaling. We experimented with four types of augmented images:
\begin{equation}
\begin{aligned}
I_1 &= I \\
I_2 &= \max\left(0, I * 
\begin{bmatrix}
  0 & -1 & 0 \\
 -1 &  5 & -1 \\
  0 & -1 & 0
\end{bmatrix} \right) \\
I_3 &= b(I^3, 9)^{1/3} \\
I_4 &= \sqrt{b(I^2, 3) - b(I, 3)^2}, \\
I_5 &= \frac{1}{8} \sum_{i = -1}^{1} \sum_{j = -1}^{1} \left| I(m,n) - I(m+i, n+j) \right|
\end{aligned}
\end{equation}
where \( I_1 \) is the original image \( I \), \( I_2 \) is the high-pass filtered version enhancing edges with a Laplacian-like filter and ensuring non-negative values via \(\max(0, \cdot)\), \( I_3 \) is the cube root of a blurred cubic version of \( I \) with \( b(I^3, 9) \) representing a 9-pixel neighborhood blur, \( I_4 \) is the local standard deviation computed as the square root of the difference between the blurred squared intensity \( b(I^2, 3) \) and the square of the blurred intensity \( b(I, 3)^2 \), and \( I_5 \) is the average absolute deviation of a pixel from its $3\times3$ neighbors, calculated as the mean of absolute differences.

The experimental results, presented in Table \ref{da}, indicate that when the model is provided with histograms from four different types of augmented images, there is a noticeable improvement in performance. However, this enhancement comes at the cost of reduced processing speed. After balancing both performance and efficiency, the combination of \( I + I_5 \) emerges as the most optimal approach.

\begin{table}[ht]
\resizebox{1\linewidth}{!}{
\setlength{\tabcolsep}{2.6pt}
\begin{tabular}{lccccc}
\hline
\multicolumn{1}{c}{}               & Mean & Med. & Best 25\% & Worst 25\% & Time(ms) \\ \hline
\multicolumn{1}{l|}{I}             & 2.31 & 2.03 & 0.57      & 6.14       & -        \\
\multicolumn{1}{l|}{I+I2}          & 2.04 & 1.84 & 0.46      & 5.18       & \cellcolor{yellow!60}\textbf{4.9}      \\
\multicolumn{1}{l|}{I+I3}          & 2.07 & 1.88 & 0.48      & 5.29       & 11.3     \\
\multicolumn{1}{l|}{I+I4}          & 2.09 & 1.92 & 0.49      & 5.31       & 13.8     \\
\multicolumn{1}{l|}{I+I5}          & 1.98 & 1.79 & 0.42      & 4.91       & 6.2      \\
\multicolumn{1}{l|}{I+I2+I3+I4+I5} & \cellcolor{yellow!60}\textbf{1.90} & \cellcolor{yellow!60}\textbf{1.74} & \cellcolor{yellow!60}\textbf{0.40}      & \cellcolor{yellow!60}\textbf{4.79}       & 35.7     \\ \hline
\multicolumn{1}{c}{}               &      &      &           &            &         
\end{tabular}
}
\caption{The effect of different data augmentations on model performance. Experiments were conducted on the LSMI Galaxy dataset, with window and overlap sizes set to 128 and 64, respectively.}
\label{da}
\end{table}

\section{Histogram Features}
In the main paper, we set the number of bins to 64. Next, we will investigate the impact of varying bin sizes on the experimental results. The experiments are conducted on the LSMI Galaxy dataset, using two histograms as input: (1) the pixel intensity distribution in log-chroma space (\( I_1 \)), and (2) the gradient intensity histogram \( I_5 \). To ensure that the data distribution within the dataset is fully contained within the defined \( u \) and \( v \) bounds, the range of \( u \) and \( v \) was set to \([-2.525, 2.525]\).

The experimental results, as shown in the Table\ref{hf}, demonstrate that when the number of bins \(n\) is too small, the color distribution is overly simplified, leading to a reduction in the amount of color detail captured by the model. This, in turn, hampers the model's ability to accurately recover true colors under diverse lighting conditions. Conversely, when \(n\) is too large, model performance tends to degrade. The increased number of bins may capture more noise than meaningful information. Furthermore, an excessive number of bins can lead to data sparsity, especially in smaller datasets, where each bin contains less information, thereby affecting the model's feature extraction capabilities.

\begin{table}[h]
\centering
\resizebox{0.97\linewidth}{!}{
\setlength{\tabcolsep}{2.6pt}

\begin{tabular}{ccccc}
\cline{2-5}
                           & Mean & Med. & \begin{tabular}[c]{@{}c@{}}Best\\ 25\%\end{tabular} & \begin{tabular}[c]{@{}c@{}}Worst\\ 25\%\end{tabular} \\ \hline
\multicolumn{1}{c|}{n=16}  & 2.79 $\pm$ 0.01 & 2.39 $\pm$ 0.01 & 0.90 $\pm$ 0.01                                                & 5.47 $\pm$ 0.01                                                 \\
\multicolumn{1}{c|}{n=32}  & 2.17 $\pm$ 0.01 & 1.84 $\pm$ 0.01 & 0.51 $\pm$ 0.01                                                & 4.98 $\pm$ 0.01                                                 \\
\multicolumn{1}{c|}{n=64}  & \cellcolor{yellow!60}1.98$\pm$ 0.01 & \cellcolor{yellow!60}1.79$\pm$ 0.01 & 0.42$\pm$ 0.01                                                & \cellcolor{yellow!60}4.91$\pm$ 0.01                                                 \\
\multicolumn{1}{c|}{n=128} & 2.19$\pm$ 0.01 & 1.81$\pm$ 0.01 & \cellcolor{yellow!60}0.41$\pm$ 0.01                                                & 5.05$\pm$ 0.01                                                 \\ \hline
\end{tabular}
}
\caption{Impact of varying bin numbers \(n\) on model performance.}
\label{hf}
\end{table}

\section{Extensions of IFFCC}
In the main paper, we learned a set of weights that determine the shape of the filters used in frequency-domain convolution, as well as the gain and bias of those filters. Here, we extend IFFCC by learning a mapping from each training sample \( x_i \) to a set of weights \( w_i \), rather than learning a single model. We optimize the weights in a small neural network with a ReLU activation function. Similar to other experiments, we use L-BFGS for training; however, the 'pretraining phase' from previous experiments is removed, and we train for 64 iterations only. The network weights are initialized with random Gaussian noise, and the weights \( w \) are indirectly regularized during the training process. This network-based methodology enhances the model's capability to infer information beyond simple pixel and edge log-chroma histograms, incorporating higher-level features such as semantic information and camera metadata.

To obtain additional information from images (metadata), we conducted experiments on the Shadow dataset, which includes metadata for each image captured by different cameras, such as exposure time and aperture size. When the network is aware that the images come from two different sensors, it can better handle the mapping relationships. Exposure time and similar metadata provide useful cues for distinguishing between ambient light and artificial light sources. Experimental results demonstrate that these metadata features are highly informative, significantly improving model performance and reducing error. We encode the additional information as a feature vector:
\begin{equation}
\begin{aligned}
    E &= \text{vec}\left( [\log(A); \log(B); \log(C); 1; 1] \right) \times \mathbf{e}_i \\
    \mathbf{e}_i &= [0, \dots, 0, 1, 0, \dots, 0] \in \mathbb{R}^N
\end{aligned}
\end{equation}
where \( A \) represents the shutter speed, \( B \) represents the image's f-number, and \( C \) represents the ISO.
The \( i \)-th element of \( \mathbf{e}_i \) is 1, with the remaining elements being 0, representing the name of the \( i \)-th camera.

We performed experiments using the nighttime scene from the Shadow dataset, which contains images captured by five distinct cameras. As demonstrated in the table, incorporating additional metadata (such as shutter speed, ISO, aperture size, and camera name) into the neural network significantly enhanced the model's performance. This improvement can be attributed to the fact that the sensor characteristics and exposure settings of different cameras have a substantial effect on the color and brightness of the images. By integrating this metadata, the model is better equipped to comprehend and adapt to the shooting conditions of various cameras, resulting in more accurate color restoration, particularly under diverse lighting conditions. Furthermore, the metadata offers valuable contextual information regarding the camera and shooting environment, thereby facilitating more effective color correction and color recovery. As a result, the inclusion of this metadata substantially boosts the model's overall performance.
However, when the network depth was increased, we observed a slight decrease in performance, which may be attributed to overfitting.

\begin{table}[ht]
\resizebox{1\linewidth}{!}{
\setlength{\tabcolsep}{2.6pt}
\begin{tabular}{cccccc}
\hline
    &                                 & Mean & Med. & Best 25\% & Worst 25\% \\ \hline
- & \multicolumn{1}{c|}{base}      & 2.85 & 1.53 & 0.54      & 7.43       \\
L=2 & \multicolumn{1}{c|}{deep+A}     & 2.69 & 1.50 & 0.54      & 6.93       \\
L=2 & \multicolumn{1}{c|}{deep+B}     & 2.71 & 1.52 & 0.53      & 6.94       \\
L=2 & \multicolumn{1}{c|}{deep+C}     & 2.66 & 1.51 & 0.53      & 6.86       \\
L=2 & \multicolumn{1}{c|}{deep+A+B+C} & \cellcolor{yellow!60}\textbf{2.56} & \cellcolor{yellow!60}\textbf{1.47} & \cellcolor{yellow!60}\textbf{0.52}     & \cellcolor{yellow!60}\textbf{6.52}       \\
L=4 & \multicolumn{1}{c|}{deep+A+B+C} & 2.65 & 1.50 & 0.56      & 6.82       \\
L=6 & \multicolumn{1}{c|}{deep+A+B+C} & 2.69 & 1.53 & 0.57      & 6.88       \\ \hline
\end{tabular}
}
\caption{Variants of IFFCC. 'deep' indicates the use of a network to learn a set of parameters, where 'L' represents the number of layers, and 'A', 'B', 'C' correspond to different types of encoded additional information. The number of hidden neurons in each layer of the network is set to 4.}
\label{deep}
\end{table}

\section{More Visual}
To further highlight the effectiveness of our method, we present additional visual comparison results in the supplementary materials. These results cover a range of challenging scenarios, including complex lighting conditions, diverse color distributions, and intricate spatial arrangements, as illustrated in Fig. \ref{s3}, Fig. \ref{s1} and Fig. \ref{s2}.

\begin{figure*}
    \centering
    \includegraphics[width=1\linewidth]{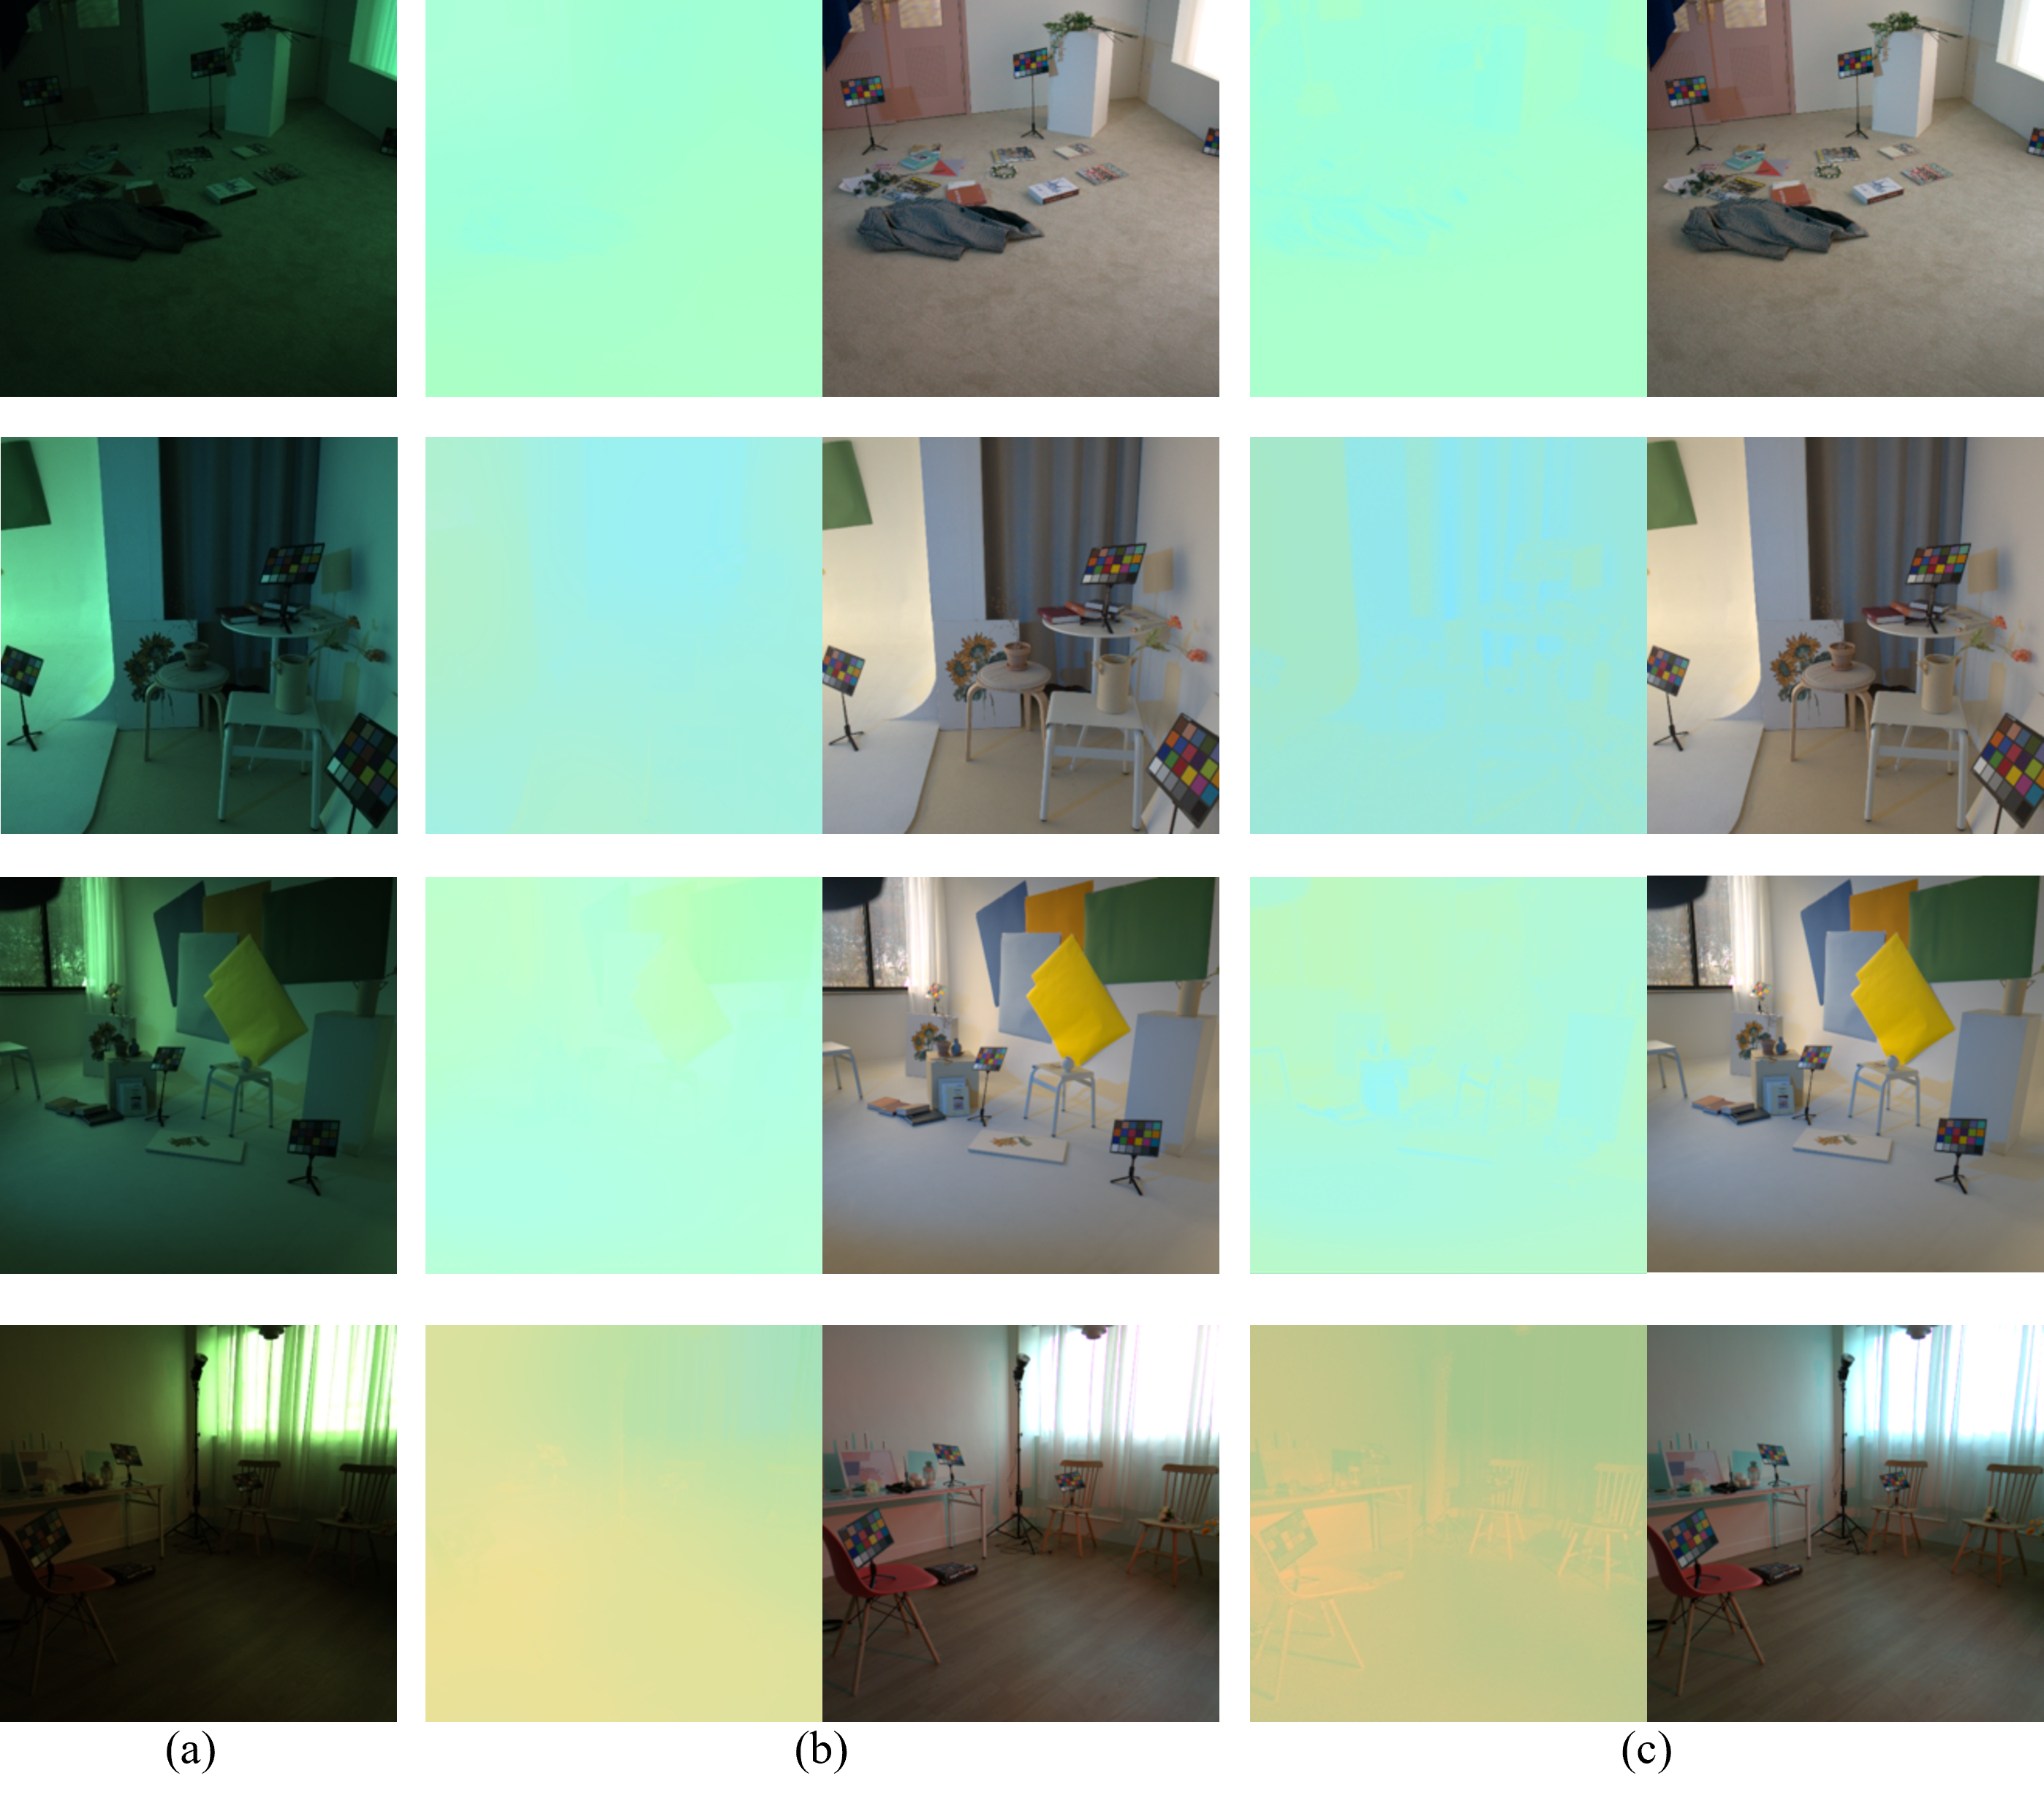}
    \caption{More visual results on the LSMI dataset. (a) represents the input RAW image, (b) shows the illumination map and white-balanced image predicted by our model (both visualized after color correction and gamma correction for better clarity), and (c) depicts the ground-truth illumination map and white-balanced image (also visualized after color correction and gamma correction). The window size and overlap size for IFFCC are set to 32 and 16, respectively.}
    \label{s3}
\end{figure*}

\begin{figure*}
    \centering
    \includegraphics[width=1\linewidth]{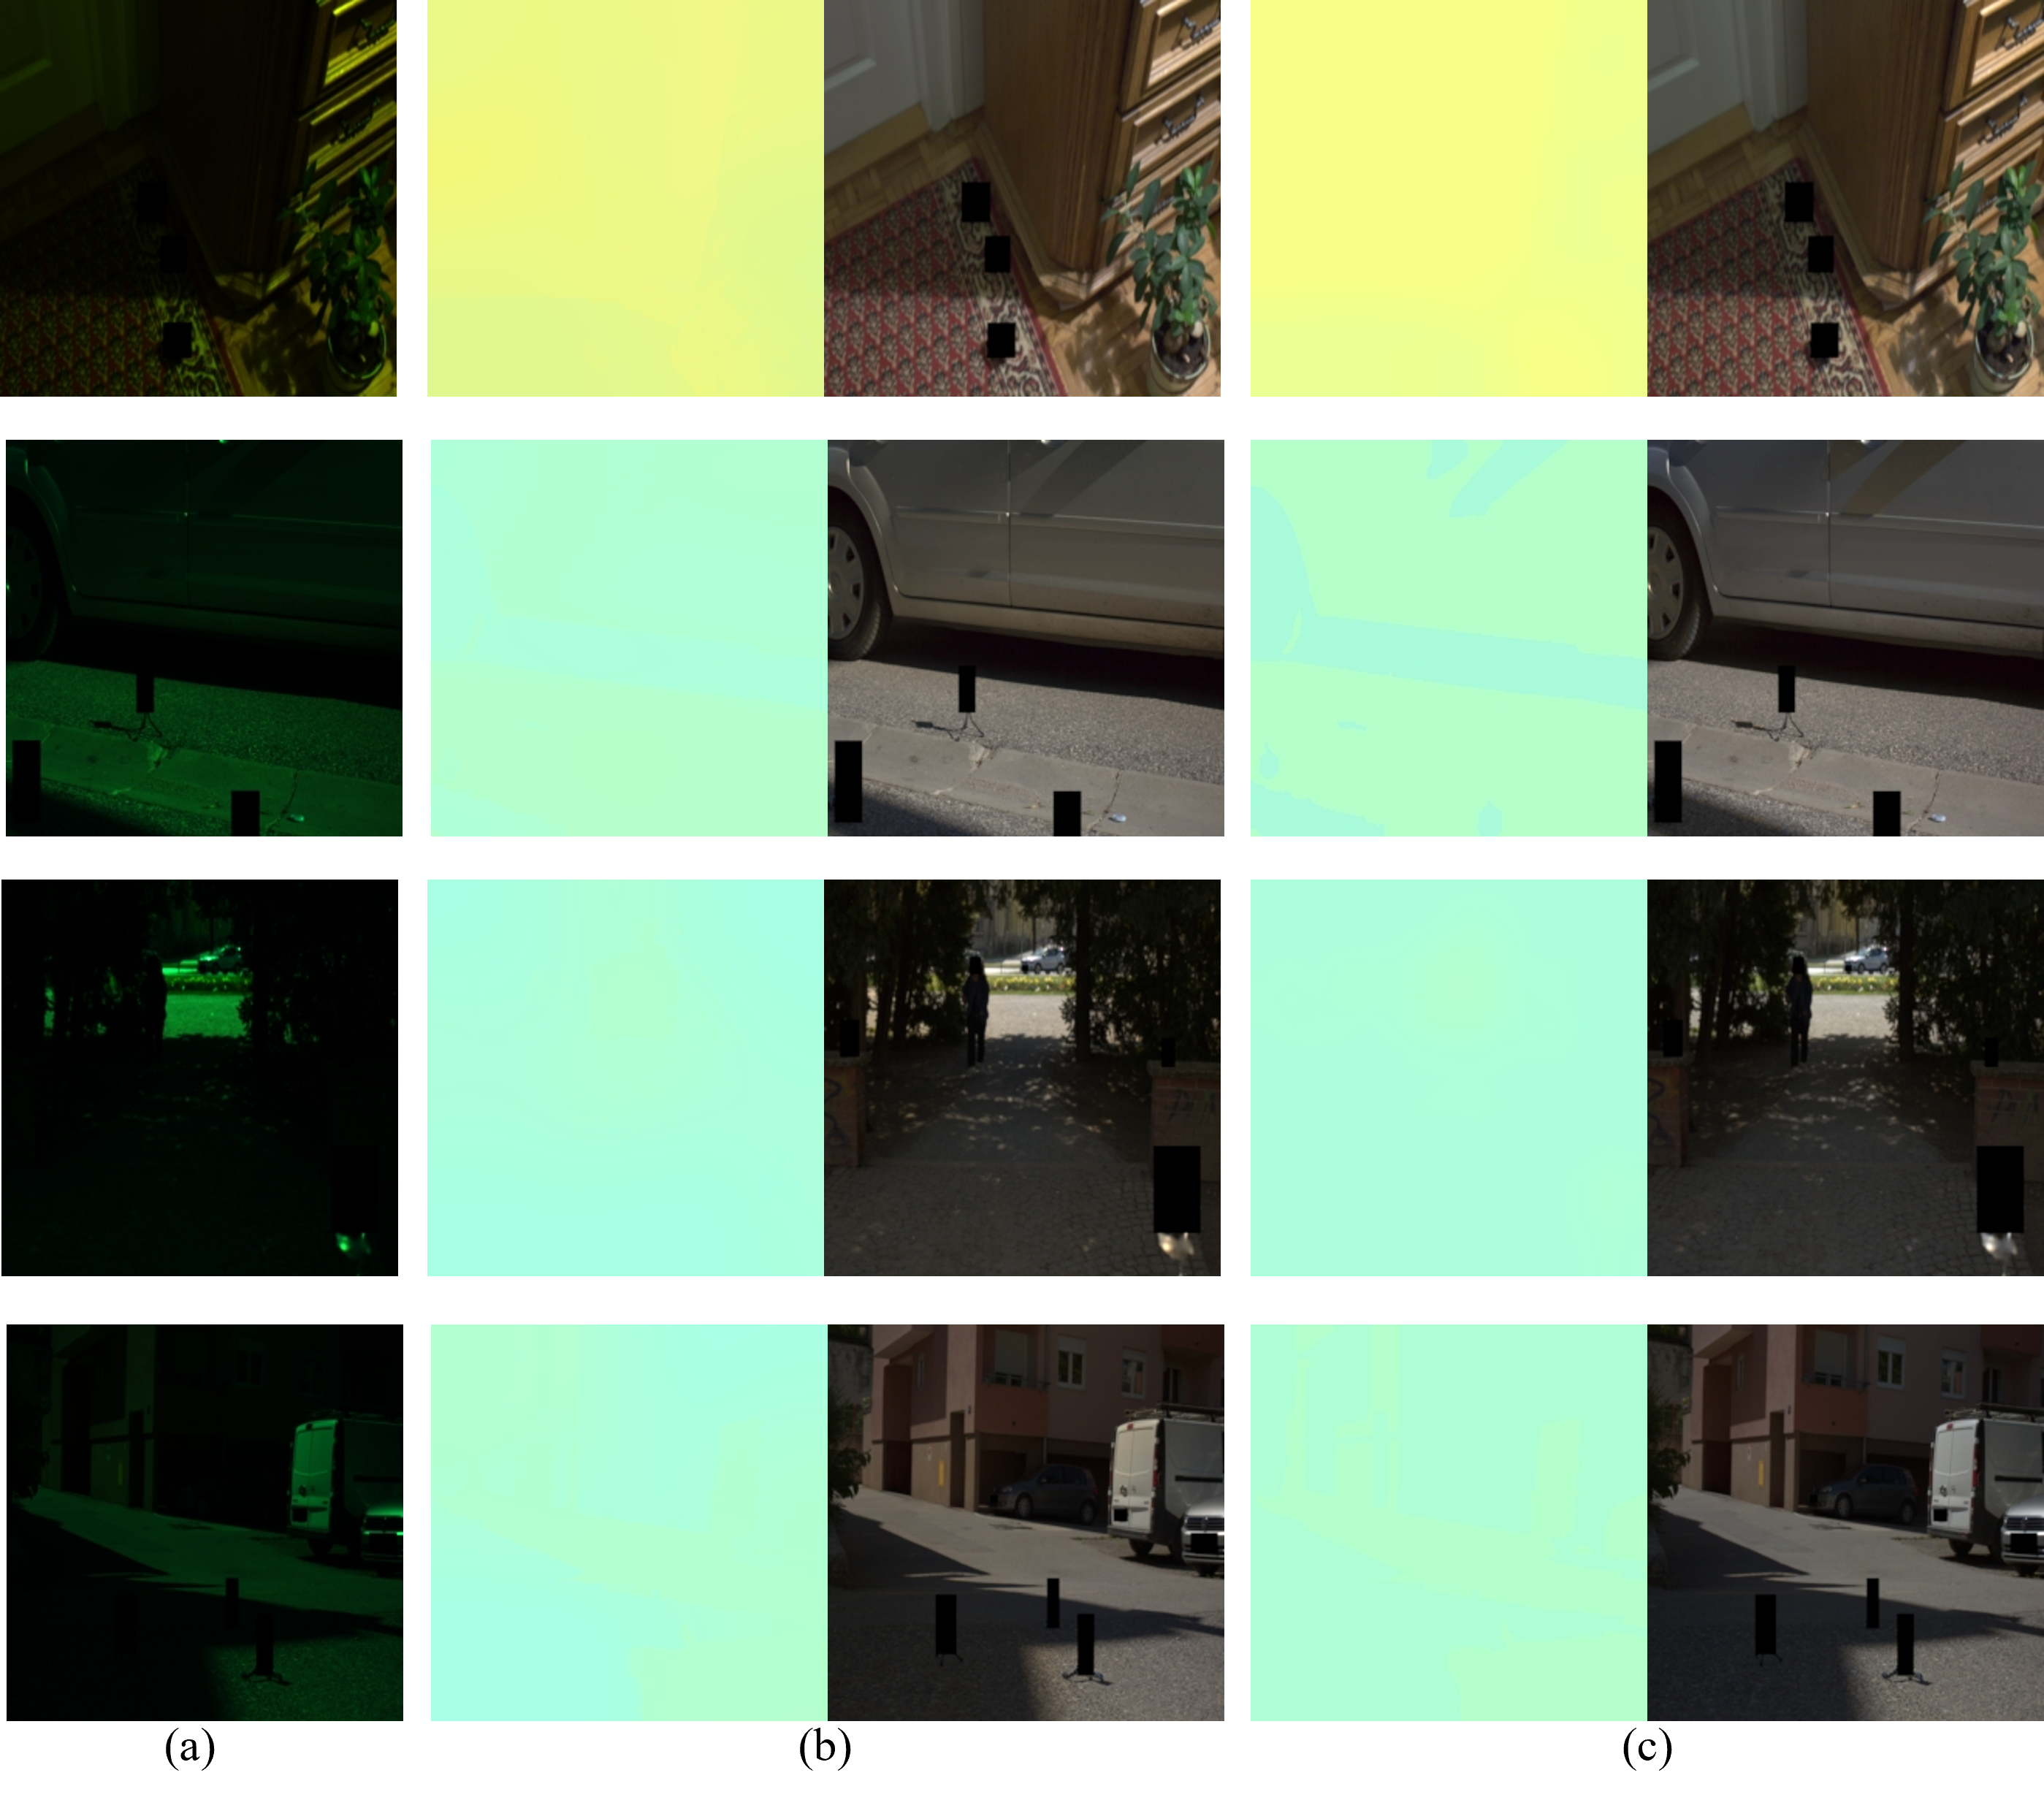}
    \caption{More visual results on the Shadow dataset. (a) represents the input RAW image, (b) shows the illumination map and white-balanced image predicted by our model (both visualized after color correction and gamma correction for better clarity), and (c) depicts the ground-truth illumination map and white-balanced image (also visualized after color correction and gamma correction). The window size and overlap size for IFFCC are set to 32 and 16, respectively.}
    \label{s1}
\end{figure*}

\begin{figure*}
    \centering
    \includegraphics[width=1\linewidth]{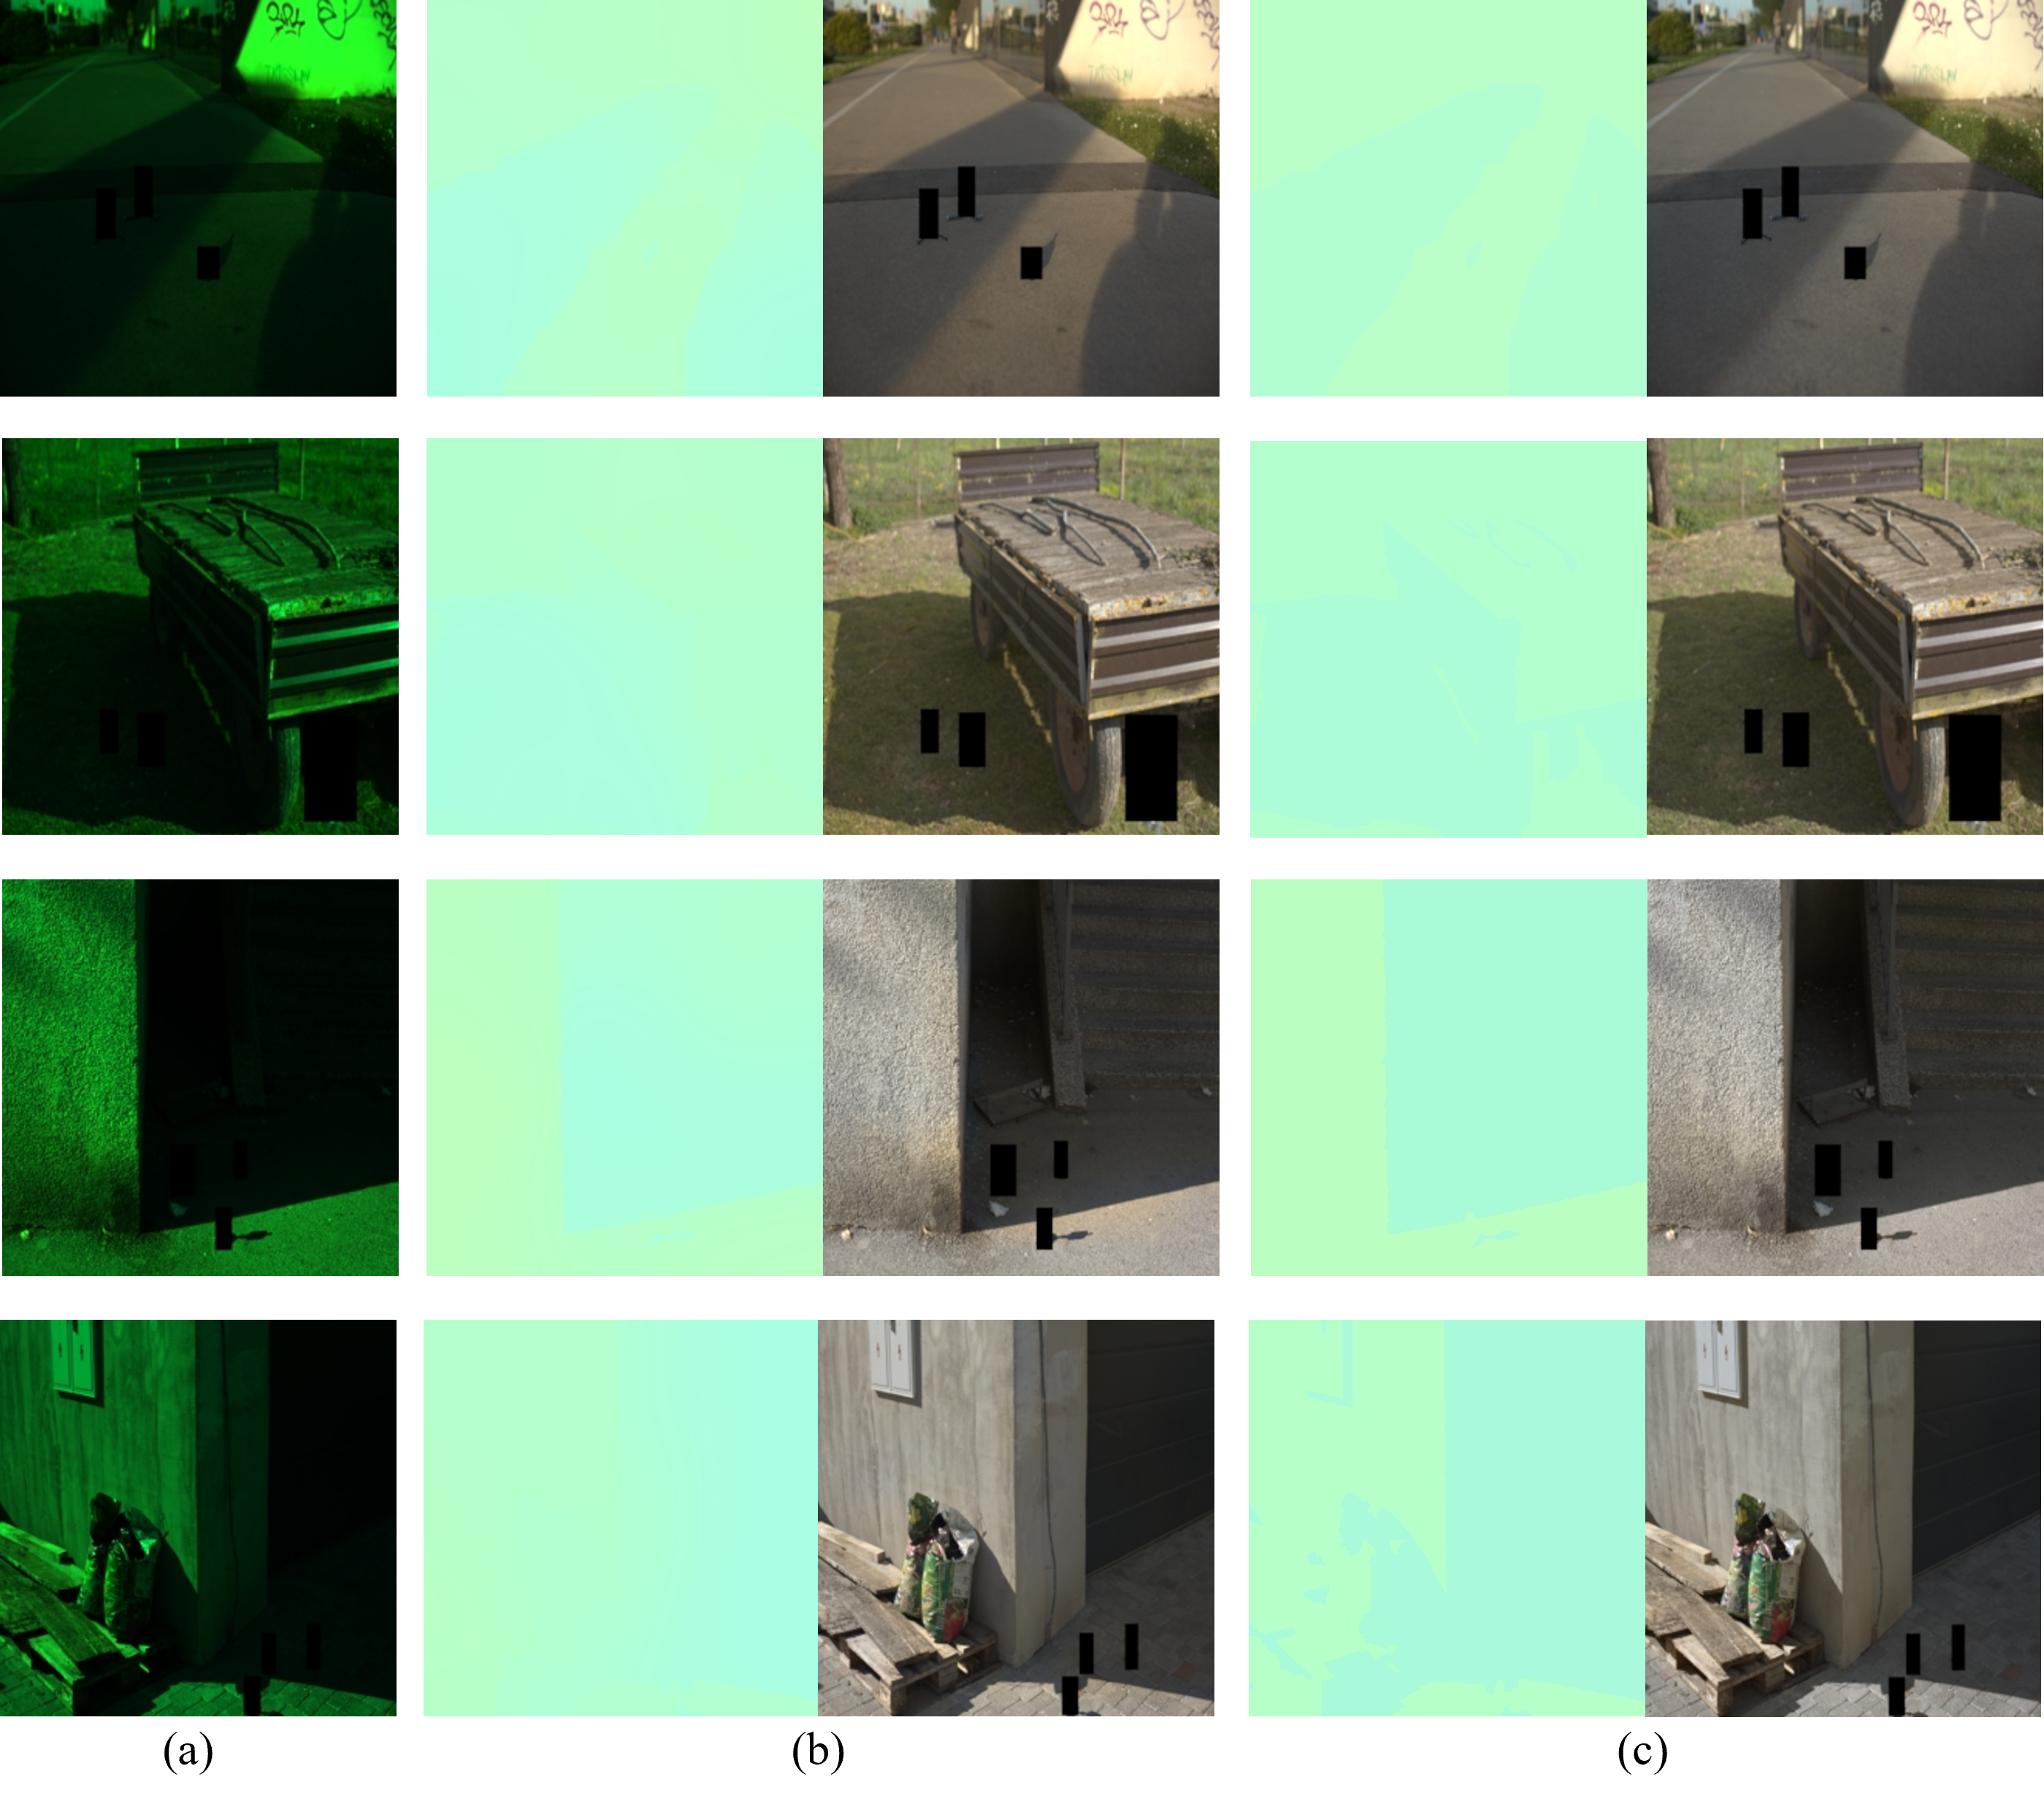}
    \caption{More visual results on the Shadow dataset. (a) represents the input RAW image, (b) shows the illumination map and white-balanced image predicted by our model (both visualized after color correction and gamma correction for better clarity), and (c) depicts the ground-truth illumination map and white-balanced image (also visualized after color correction and gamma correction). The window size and overlap size for IFFCC are set to 32 and 16, respectively.}
    \label{s2}
\end{figure*}

% \label{sec:rationale}
% % 
% Having the supplementary compiled together with the main paper means that:
% % 
% \begin{itemize}
% \item The supplementary can back-reference sections of the main paper, for example, we can refer to \cref{sec:intro};
% \item The main paper can forward reference sub-sections within the supplementary explicitly (e.g. referring to a particular experiment); 
% \item When submitted to arXiv, the supplementary will already included at the end of the paper.
% \end{itemize}
% % 
% To split the supplementary pages from the main paper, you can use \href{https://support.apple.com/en-ca/guide/preview/prvw11793/mac#:~:text=Delete%20a%20page%20from%20a,or%20choose%20Edit%20%3E%20Delete).}{Preview (on macOS)}, \href{https://www.adobe.com/acrobat/how-to/delete-pages-from-pdf.html#:~:text=Choose%20%E2%80%9CTools%E2%80%9D%20%3E%20%E2%80%9COrganize,or%20pages%20from%20the%20file.}{Adobe Acrobat} (on all OSs), as well as \href{https://superuser.com/questions/517986/is-it-possible-to-delete-some-pages-of-a-pdf-document}{command line tools}.
